# Supplementary material for: Experimental Realization of Room Temperature Topological Hall Effect in Kagome Antiferromagnet
Source: arXiv:2112.15409 source file (2023-01-31)
Supplement: Supplementary file 1 [file Mn3Sn_Supple.pdf]

# Experimental Observation of Room Temperature Topological Hall Effect in Kagome Antiferromagnet

Achintya Low, Susanta Ghosh, Sayan Routh, and Setti Thirupathaiah*
*Department of Condensed Matter and Materials Physics,*
*S . N. Bose National Centre for Basic Sciences, JD Block, Sector 3, Salt Lake, Kolkata-700106*

## EXPERIMENTAL DETAILS

For the growth of Fe doped single crystals, we followed the same method by adding the desired amount of iron powder (Alfa Aesar, 99.99%) to the Mn-Sn mixture. In this way, we obtained several shiny hexagonal-rod-shaped single crystals with typical dimensions of 2×1×1 $mm^3$. Powder X-ray diffraction (XRD) was performed using Rigaku SmartLab 9kW Cu $K_\alpha$ X-ray source. Stoichiometry of the crystals were found to be $Mn_{2.95(1)}Sn_{1.05(1)}$ and $Mn_{2.76(1)}Fe_{0.21(1)}Sn_{1.03(1)}$ using Energy Dispersive X-ray Spectroscopy (EDXS). From the EDXS data, we can observe that both compounds have marginally higher Sn concentrations. For simplicity, we denote the compositions as $Mn_3Sn$ and $Mn_{2.8}Fe_{0.2}Sn$. Electrical transport and Hall effect measurements were performed using the four-probe technique. Copper leads were attached to the sample using EPO-TEK H21D silver epoxy. Temperature-dependent resistivity data were recorded from physical properties measurement system (PPMS, Dynacool, Quantum Design) within the temperature range of 2-350 K. Hall measurements were done by sweeping the magnetic fields between -4 T and 4 T. Magnetic properties studies were done using the vibrating sample magnetometer (VSM) option of PPMS (Dynacool, Quantum Design) within the temperature range of 2-350 K and magnetic field was varied between -4 T and 4 T.

The powder XRD pattern of the crushed single crystals shown in the bottom panel of Figure 1(a) in the main text confirms that $Mn_3Sn$ crystalizes into hexagonal phase with a space group of $P6_3/mmc$ (194). No impurity peaks have been detected from the XRD pattern, which suggests pure-phase $Mn_3Sn$ single crystals. From the XRD pattern refinement of $Mn_3Sn$ we obtain lattice parameters $a$=$b$= 5.679(2) $\AA$ and $c$=4.533(4) $\AA$ which are comparable to the reported values of $Mn_3Sn$ [1, 2]. The XRD patterns have taken on the single crystals of $Mn_3Sn$ and $Mn_{2.8}Fe_{0.2}Sn$ show multiple reflections corresponding to (0002) and (0004) planes.

## MAGNETIC PROPERTIES

Magnetization as a function of temperature M(T), plotted for zero-field cooling (ZFC) and field cooling (FC) modes with an external magnetic field of 500 Oe applied parallel and perpendicular to $c$-axis is shown in Fig. 1(a) for $Mn_3Sn$ and in Fig. 1(b) for $Mn_{2.8}Fe_{0.2}Sn$. When the field is applied perpendicular to $c$-axis ($H \perp c$), in $Mn_3Sn$, a huge drop in magnetization is noticed at 260 K for both FC and ZFC modes, while the magnetization drop still present for the field applied parallel to $c$-axis ($H \parallel c$) but relatively small compared to $H \perp c$. The magnetization drop at 260 K for $H \perp c$ can be understood as a result of spin-reorientation from inverse-triangular to spin-spiral structure [3–8]. Further reduction in temperature leads to spin-glass transition at 40 K as we find a cusp-like splitting in the magnetization

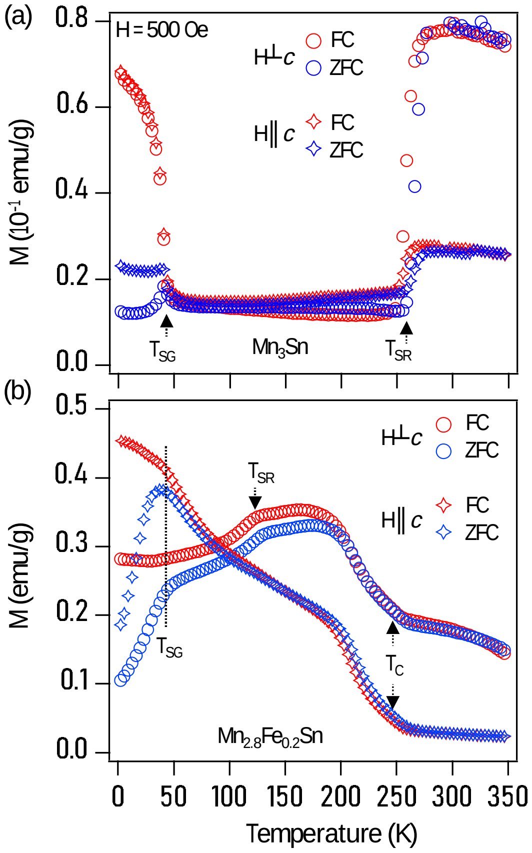


Figure 1. Magnetization as a function of temperature, M(T), plotted for $Mn_3Sn$ (a) and $Mn_{2.8}Fe_{0.2}Sn$ (b). In figures, $T_{SR}$ is spin reorientation transition temperature, $T_{SG}$ is spin-glass transition temperature, and $T_C$ is Curie-Weiss temperature. The data is collected with an external magnetic field of 500 Oe applied both in parallel and perpendicular to the $c$-axis.

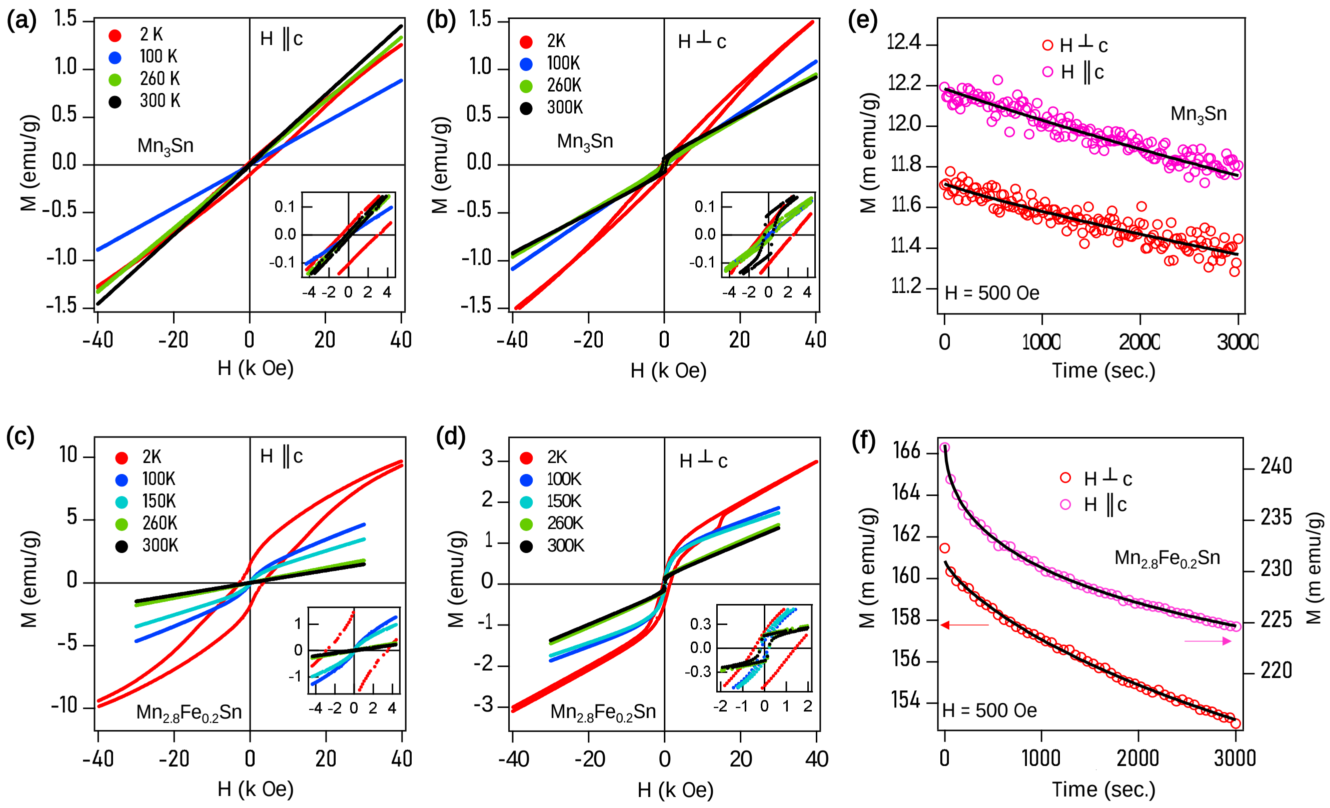


Figure 2. Magnetization isotherms, M(H), of $Mn_3Sn$ for field applied parallel (a) and perpendicular (b) to the $c$-axis measured at various temperatures. Similarly, magnetization isotherms of $Mn_{2.8}Fe_{0.2}Sn$ for field applied parallel (c) and perpendicular (d) to the $c$-axis measured at various temperatures. (e) and (f) show magnetization relaxation data plotted as a function of time, measured at 5 K with an external field of 500 Oe applied parallel and perpendicular to the $c$-axis from $Mn_3Sn$ and $Mn_{2.8}Fe_{0.2}Sn$, respectively.

curve between ZFC and FC modes as shown in Fig. 1(a). Quantitative comparison of our $Mn_3Sn$ magnetization data with the existing literature is quite challenging as the magnetic properties of this system are highly sensitive to the growth conditions and the chemical compositions [9]. However, the spin-reorientation and spin-glass transitions are inline with the previous reports [3, 5, 7, 8].

For a better understanding of the magnetism of these systems, we performed isothermal magnetization M(H) measurements as shown in figure 2. Figs. 2 (a) and 2 (b) depict M(H) isotherms from $Mn_3Sn$ for $H \| c$ and $H \perp c$, respectively. From Fig. 2 (a), we see significant magnetic hysteresis in $Mn_3Sn$ for $H \| c$ at 2 K without saturation even at an applied field of 4 T. But at higher temperatures, the magnetic hysteresis disappears. The observed magnetic hysteresis at 2 K is possibly due to short-range magnetic ordering due to spin fluctuations in the spin-glass state. As shown in Fig. 2 (b), for $H \perp c$ also the isotherms M(H) are found to be similar to $H \| c$ with significant magnetic hysteresis at 2 K again due to glassy spin nature. In contrast, we find a weak ferromagnetic-like hysteresis with large coercivity and remanence at 300 K. Moreover, the slope dM/dH obtained at higher fields ($> 3$ T) decreases with increasing temperature, hinting at reduced antiferromagnetism in $Mn_3Sn$ at higher temperatures. Therefore, we conclude that the observed magnetic hysteresis at low temperatures for both $H \perp c$ and $H \| c$ in $Mn_3Sn$ is due to the short-range magnetic interactions below $< 40$ K. The anisotropic magnetization between $H \perp c$ and $H \| c$ in $Mn_3Sn$ is in good agreement with previous magnetic studies on $Mn_3Sn$ [1].

Figures 2(c) and 2(d) depict M(H) isotherms measured on $Mn_{2.8}Fe_{0.2}Sn$ at various temperatures for both $H \| c$ and $H \perp c$, respectively. From Fig. 2(c), for $H \| c$, we can see that the Fe doping induces a long-range ferromagnetic ordering as the magnetic hysteresis is found with increased coercivity at 2 K. But the magnetic hysteresis disappears at temperatures of 100 and 150 K, while still having a sigmoid-like M(H) curve. On the other hand, at the temperatures of 260 and 300 K, we observe that the system completely transforms into antiferromagnet as we find linear M(H) isotherms. Next from Fig. 2(d), for $H \perp c$, we observe M(H) isotherm with a coercivity of 850 Oe at 2 K. Interestingly, we also notice a field-induced asymmetric M(H) curve at 2 K that is not visible for $H \| c$. We further observe reduced coercivity of 220 Oe at

260 K, which is nearly constant up to 300 K without any field-induced asymmetry in the M(H) loop. Note here that the coercivity of $Mn_{2.8}Fe_{0.2}Sn$ is almost a factor of 2 less compared to the parent system for H$\perp c$ at 300 K. Whereas, the coercivity of $Mn_{2.8}Fe_{0.2}Sn$ is nearly 2 times higher compared to $Mn_3Sn$ at 2 K for H$\|c$.

The glassy-spin nature of the systems is further examined by performing magnetization relaxation measurements for both $Mn_3Sn$ and $Mn_{2.8}Fe_{0.2}Sn$ as shown in Figs. 2(e) and 2(f), respectively, measured with an applied magnetic field of 500 Oe in the FC mode at 5 K. Magnetization relaxation for a spin-glass system can be explained using the Stretched function, $M(t) = A\ exp[-(\frac{t}{\tau})^{\alpha}]$ [10]. Here, $A$ is an exponential factor, $t$ is the time, $\tau$ is a characteristic relaxation time constant, and $\alpha$ is stretching exponent which is temperature dependent and can take the values $0 < \alpha < 1$ [11]. From the Stretched function fitting to $Mn_3Sn$ [see Fig. 2(e)], we obtain $\alpha$=0.96±0.04 and $\tau$=(1.03±0.17)$10^5$ s for H$\|c$. Similarly, $\alpha$=0.85±0.1 and $\tau$=(1.83±0.77)$10^5$ s are obtained for H$\perp c$. The $\alpha$ values close to 1 and higher relaxation time constants suggest $Mn_3Sn$ to be nearly an isotropic spin-glass system. On the other hand, the best fit for the magnetization relaxation curves from $Mn_{2.8}Fe_{0.2}Sn$ is obtained using the modified Stretched function $M(t) = M_0 + A\ exp[-(\frac{t}{\tau})^{\alpha}]$ [12–14]. Here, the additional term $M_0$ is the magnetization due to long-range ferromagnetic ordering at $t$=∞ [15]. From the fitting [see Fig. 2(f)] we obtained $M_0$= 0.21±0.1 emu/g, $\tau$=5672±512 s and $\alpha$=0.47±0.01 for H$\|c$. Similarly, we obtained $M_0$= 0.14±0.01 emu/g, $\tau$=7316.8 ± 31.9 s and $\alpha$=0.76±0.02 for H$\perp c$. Here, different $\alpha$ values (<1) for different crystal orientations found in $Mn_{2.8}Fe_{0.2}Sn$ suggest for anisotropic ferromagnetism induced with Fe doping, which is consistent with the anisotropic magnetization isotherms, M (H), shown in Figs. 2(c) and 2(d).

* setti@bose.res.in


[1] T. F. Duan, W. J. Ren, W. L. Liu, S. J. Li, W. Liu, and Z. D. Zhang, Magnetic anisotropy of single-crystalline $Mn_3Sn$ in triangular and helix-phase states, Appl. Phys. Lett. **107**, 082403 (2015).

[2] N. H. Sung, F. Ronning, J. D. Thompson, and E. D. Bauer, Magnetic phase dependence of the anomalous Hall effect in $Mn_3Sn$ single crystals, Appl. Phys. Lett. **112**, 132406 (2018).

[3] S. Tomiyoshi and Y. Yamaguchi, Magnetic Structure and Weak Ferromagnetism of Mn3Sn Studied by Polarized Neutron Diffraction, J. Phys. Soc. Japan **51**, 2478 (1982).

[4] H. Ohmori, S. Tomiyoshi, H. Yamauchi, and H. Yamamoto, Spin structure and weak ferromagnetism of $Mn_3Sn$, J. Magn. Magn. Mater. **70**, 249 (1987).

[5] J. Sticht, K.-H. Höck, and J. Kübler, Non-collinear itinerant magnetism: the case of $Mn_3Sn$, Journal of Physics: Condensed Matter **1**, 8155 (1989).

[6] P. J. Brown, V. Nunez, F. Tasset, J. B. Forsyth, and P. Radhakrishna, Determination of the magnetic structure of $Mn_3Sn$ using generalized neutron polarization analysis, J. Phys. Condens. Matter **2**, 9409 (1990).

[7] S. Nakatsuji, N. Kiyohara, and T. Higo, Large anomalous Hall effect in a non-collinear antiferromagnet at room temperature, Nature **527**, 212 (2015).

[8] P. Park, J. Oh, K. Uhlířová, J. Jackson, A. Deák, L. Szunyogh, K. H. Lee, H. Cho, H.-L. Kim, H. C. Walker, *et al.*, Magnetic excitations in non-collinear antiferromagnetic Weyl semimetal $Mn_3Sn$, npj Quantum Materials **3**, 63 (2018).

[9] E. Kren, J. Paitz, G. Zimmer, and E. Zsoldos, Study of the magnetic phase transformation in the $Mn_3Sn$ phase, Physica B+C **80**, 226 (1975).

[10] J. A. Mydosh, *Spin glasses: an experimental introduction* (CRC Press, 1993).

[11] R. V. Chamberlin, G. Mozurkewich, and R. Orbach, Time Decay of the Remanent Magnetization in Spin-Glasses, Phys. Rev. Lett. **52**, 867 (1984).

[12] P. D. Mitchler, R. M. Roshko, and W. Ruan, Non-equilibrium relaxation dynamics in the spin glass and ferromagnetic phases of CrFe, Philos. Mag. B **68**, 539 (1993).

[13] G. Sinha, R. Chatterjee, M. Uehara, and A. K. Majumdar, Relaxation of thermo-remanent magnetization in different magnetic phases of Fe-rich $\gamma$-FeNiCr alloys, J. Magn. Magn. Mater. **164**, 345 (1996).

[14] B. Pang, L. Zhang, Y. Chen, J. Zhou, S. Yao, S. Zhang, and Y. Chen, Spin-glass-like behavior and topological Hall effect in $SrRuO_3/SrIrO_3$ superlattices for oxide spintronics applications, ACS Appl. Mater. Interfaces **9**, 3201 (2017).

[15] M. Gabay and G. Toulouse, Coexistence of spin-glass and ferromagnetic orderings, Phys. Rev. Lett. **47**, 201 (1981).
